# Supplementary material for: Concentration dependence of diffusion-limited reaction rates and its consequences
Source: arXiv:2002.00485 ancillary file (2020-10-02)
Supplement: Supplementary file 1 [file SI_p12.pdf]

# Supplementary Information: Concentration dependence of diffusion-limited reaction rates and its consequences

Sumantra Sarkar
Center for Nonlinear Studies, Los Alamos National Laboratory

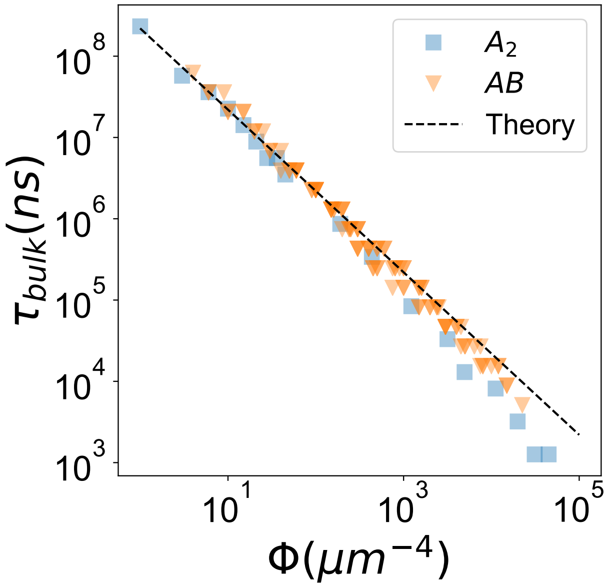


FIG. S1. $\tau_{bulk}$, the time after which diffusive collision events are Markovian, as a function of the mass-action $\Phi$. For small $\Phi$, $\tau_{bulk}$ is well approximated by $\frac{\log(L/a)}{8\pi D_A \Phi}$.

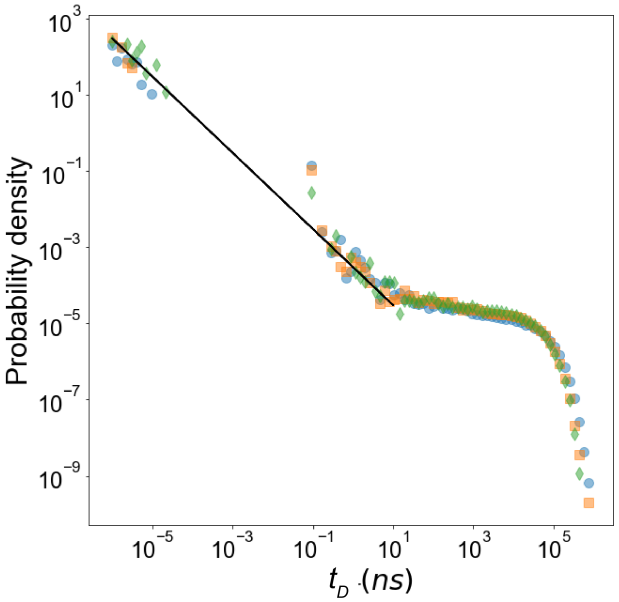


FIG. S2. Dimerization time distribution for $N = 80$ for three different experiments (three different markers) in canonical ensemble. The number of monomers and dimers were not fixed, but $[A]+2[A_2]$ was fixed at $N$. The dimerization time distribution had the same three regions as in the ensemble considered in the main text, where $[A]$ and $[A_2]$ were kept constant.

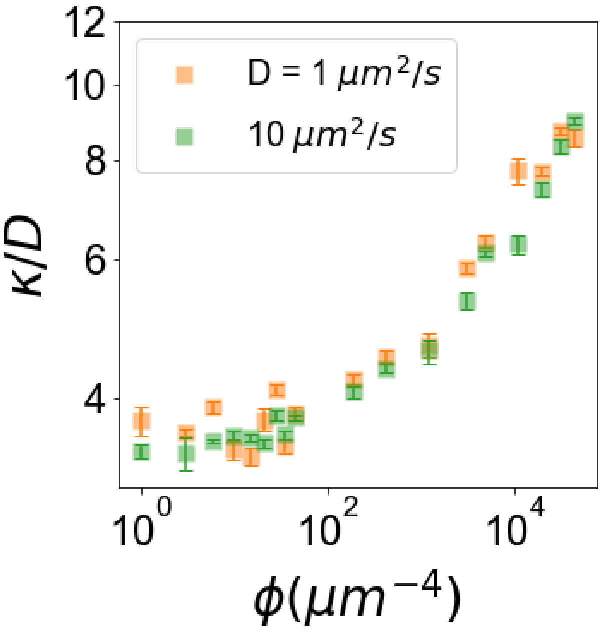


FIG. S3. Concentration dependent rate constant, $\kappa(\Phi)$ for different diffusion constants, $D$. When scaled by the diffusion constant, the reaction rates have the same scaling with $\Phi$. $r_a = 1.2 r_{min}$ was used.
